# Supplementary material for: Urban Architect: Steerable 3D Urban Scene Generation with Layout Prior
Source: arXiv:2404.06780 source file (2024-04-10)
Supplement: Supplementary file 1 [file X_suppl.tex]

\clearpage
\setcounter{page}{1}
\setcounter{section}{0}
\setcounter{figure}{0}
\setcounter{table}{0}
\setcounter{equation}{0}

\maketitlesupplementary

In this supplementary material, we provide: $(1)$ more detailed discussion on the implementation details; $(2)$  additional experimental results; 
$(3)$ the potential societal impact of our method. {\color{magenta}Our code is attached as a supplementary file and will be released.}

\section{Implementation Details}

\noindent \textbf{Details of Scalable Hash Grid.} As shown in Fig.~\ref{fig:hashgrid}, instead of modeling the entire scene using a single hash grid, we decompose the scene into a set of stuff grids ($\{\mathcal{H}_k^s\}$) and object grids ($\{\mathcal{H}_k^o\}$). Our representation is incrementally updated given the incoming camera trajectory.

\begin{figure}[htbp] % 
\centering
\includegraphics[width=1\linewidth]{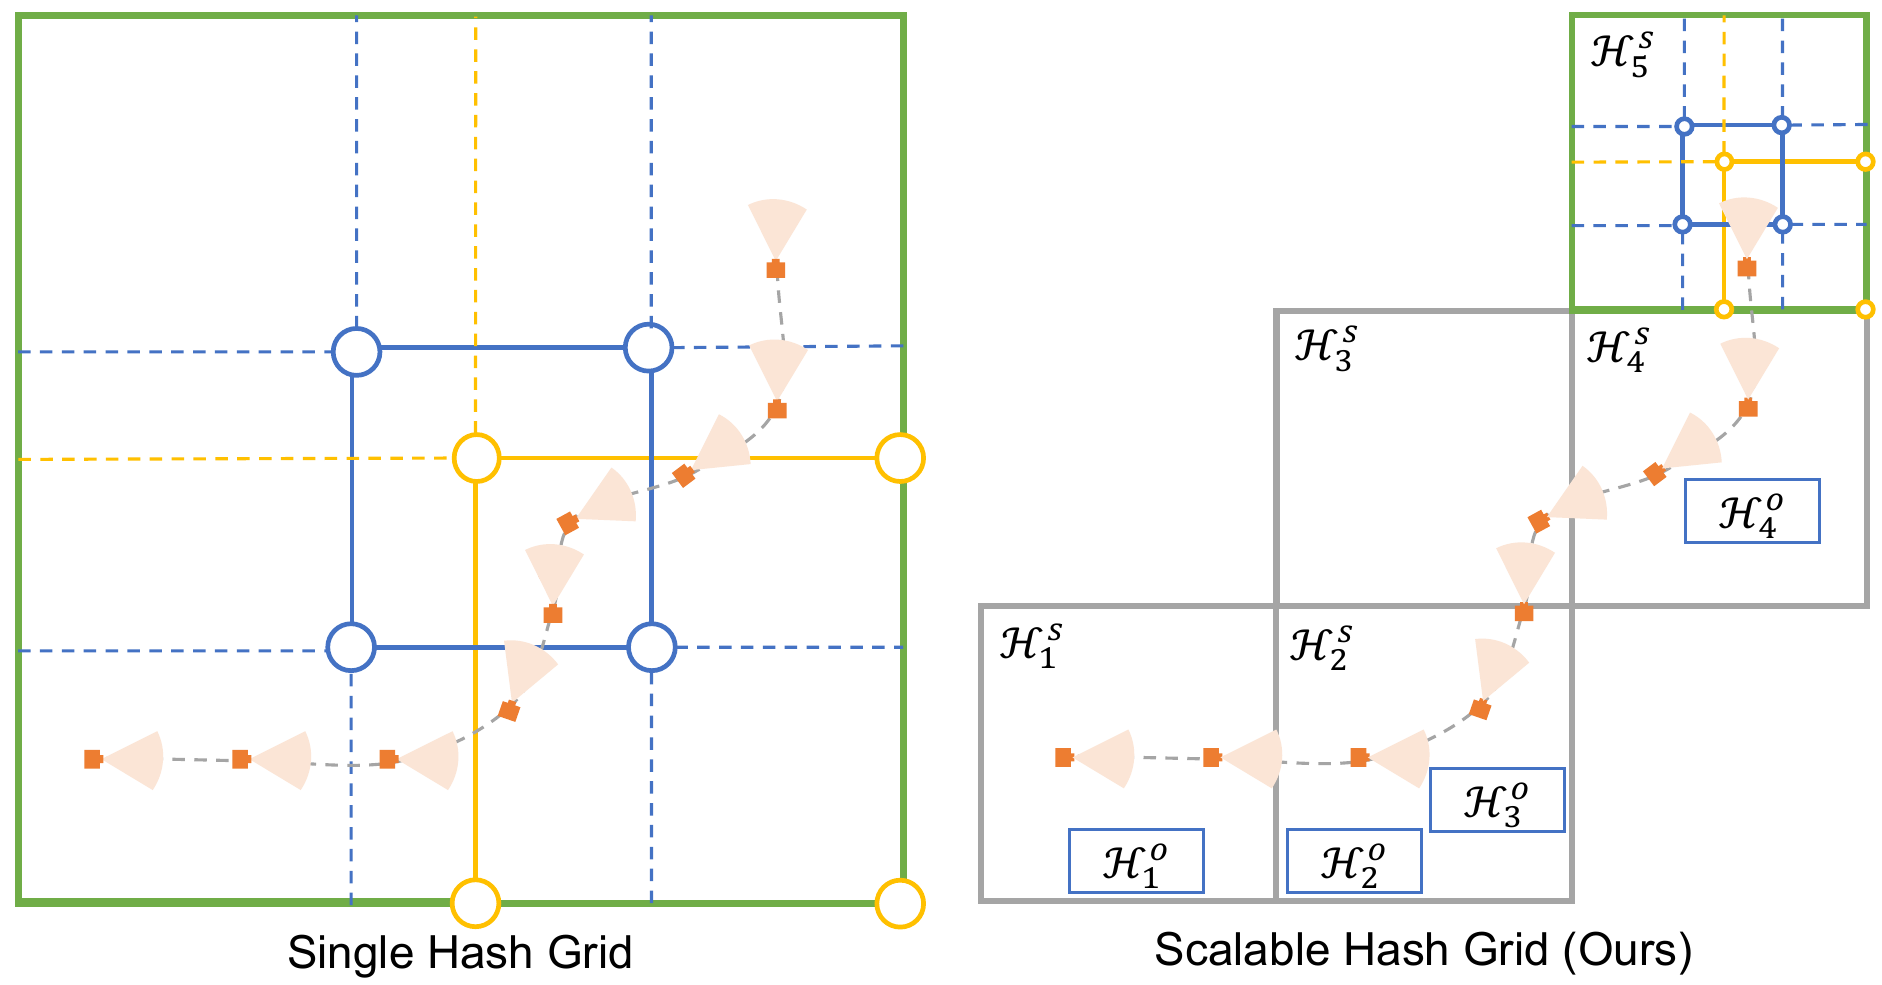}
% \vspace{-4ex}
\caption{\textbf{Illustration of the scalable hash grid representation.} We decomposed the scene into 
a set of stuff and object hash grids (\ie, $\{\mathcal{H}_k^s, \mathcal{H}_k^o\}$). The grids grow with the camera trajectory in a dynamic manner.}\label{fig:hashgrid}
% \vspace{-3ex}
\end{figure}

Based on the scalable hash grid, we can render the corresponding image given the camera pose. Given the ray $\mathbf{r}$ of a pixel, we sample a set of points $\{\mathbf{x}_i\}$ on the ray and predict the corresponding color $\{c_i\}$ and density $\{\sigma_i\}$ in the canonical space of the corresponding stuff or object grid. We model the color of the sky region using a separate MLP $\mathcal{R}_{sky}$ given the ray direction $\mathbf{d}$. The rendered pixel color $C(\mathbf{r})$ can be calculated as:
\begin{equation}
\begin{split}
    C(\mathbf{r})&=\sum_{i}^{N}T_i\alpha_i c_i + (1-\sum_{i}^{N}T_i\alpha_i)\mathcal{R}_{sky}(\mathbf{d})\\
    \alpha_i &= 1 - e^{(-\sigma_i\delta_i)},\quad T_i=\prod_{j=1}^{i-1}(1-\alpha_j).
\end{split}
\end{equation}

% \begin{equation}
%     T_i=\prod_{j=1}^{i-1}(1-\alpha_j)
% \end{equation}

\noindent \textbf{Implementation and Training.} The overall framework is implemented using PyTorch~\cite{paszke2019pytorch}. We use diffusers~\cite{diffusers} to implement the diffusion model. AdamW~\cite{loshchilov2017decoupled} is used as the optimizer with an learning rate of $1\times 10^{-3}$. For the training of ControlNet~\cite{zhang2023adding}, we concatenate the rendered semantic and depth maps from 3D layouts as the input conditional signal. We crop and resize the original image (with a resolution of $1408\times 376$ ) in the KITTI-360 dataset~\cite{liao2022kitti} to a resolution of $512\times 512$. During the refinement, we further adopt monocular depth estimation method~\cite{ranftl2020towards} to predict the depth for the rendered image and align the scale and shift with the rendered depth from the generated hash grid. We then  refine the geometry by adding an L1 error between the rendered and the aligned monocular depth. Additionally, we  employ a semantic segmentation network~\cite{jain2023oneformer} to predict sky masks and encourage the accumulated density $\alpha_i$ to converge to 0 in the sky region.

\noindent \textbf{Layout Construction.} The 3D layout representation comprises a set of semantic primitives with simple geometric structures. To ease the process of layout construction, we provide several basic primitives (as shown in Fig.~\ref{fig:primitives}), that can be easily composed to the desired scene layout.

\begin{figure}[htbp] % 
\centering
\includegraphics[width=1\linewidth]{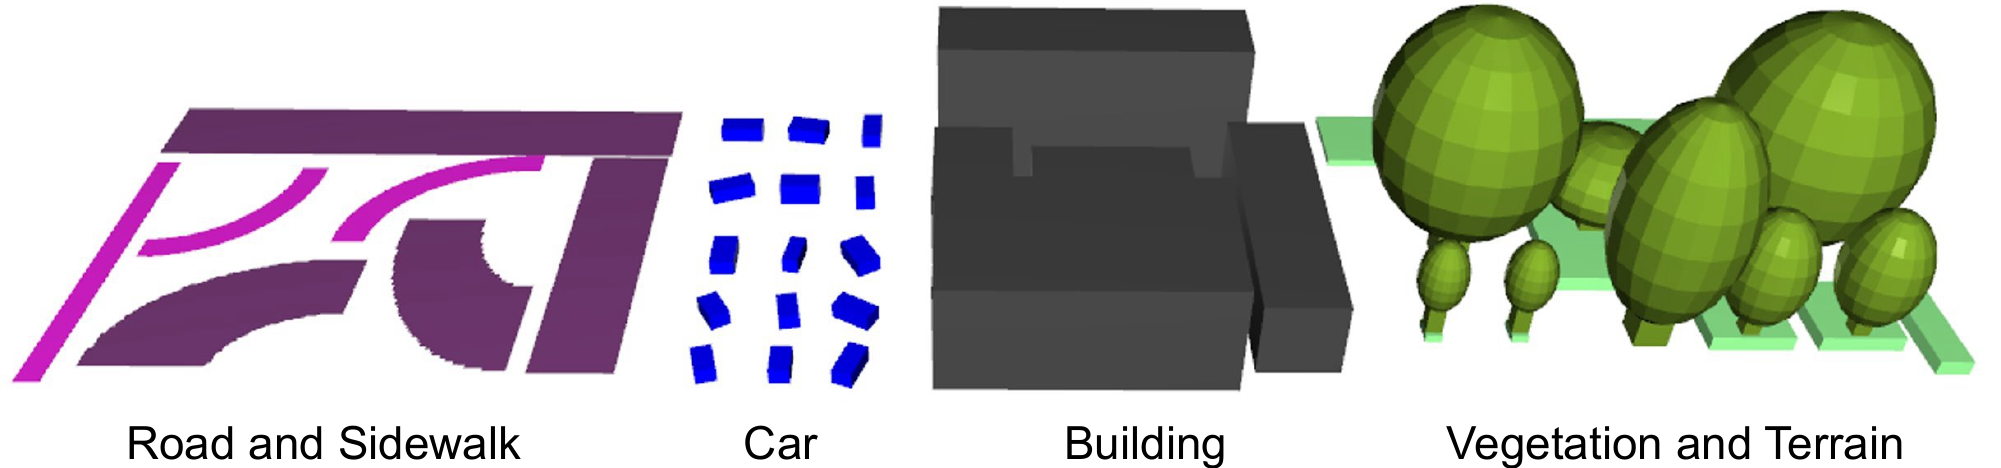}
% \vspace{-4ex}
\caption{\textbf{Basic primitives.} We provide several basic primitives of common objects in urban scenes (\eg, road and sidewalk, car, building, \etc)}\label{fig:primitives}
% \vspace{-3ex}
\end{figure}
\noindent\textbf{Automatic Layout Generation.} We further provide an alternative method to generate 3D scene layout automatically based on SinDDM~\cite{kulikov2023sinddm}. SinDDM learns the intrinsic distribution of the training image via a multi-scale diffusion process, enabling the generation of new images with arbitrary scales. Specifically, we first compress the 3D layout to the 2D ground plane and obtain a 2D representation of the 3D scene. Then, we train the SinDDM model based on the single 2D example. As shown in Fig.~\ref{fig:sinddm}, the trained model can produce diverse new samples with arbitrary scales and reasonable arrangements. We also generate scenes based on the generated 3D layouts and the rendered results are provided in the bottom row of Fig.~\ref{fig:sinddm}.

\begin{figure}[htbp] % 
\centering
\includegraphics[width=1\linewidth]{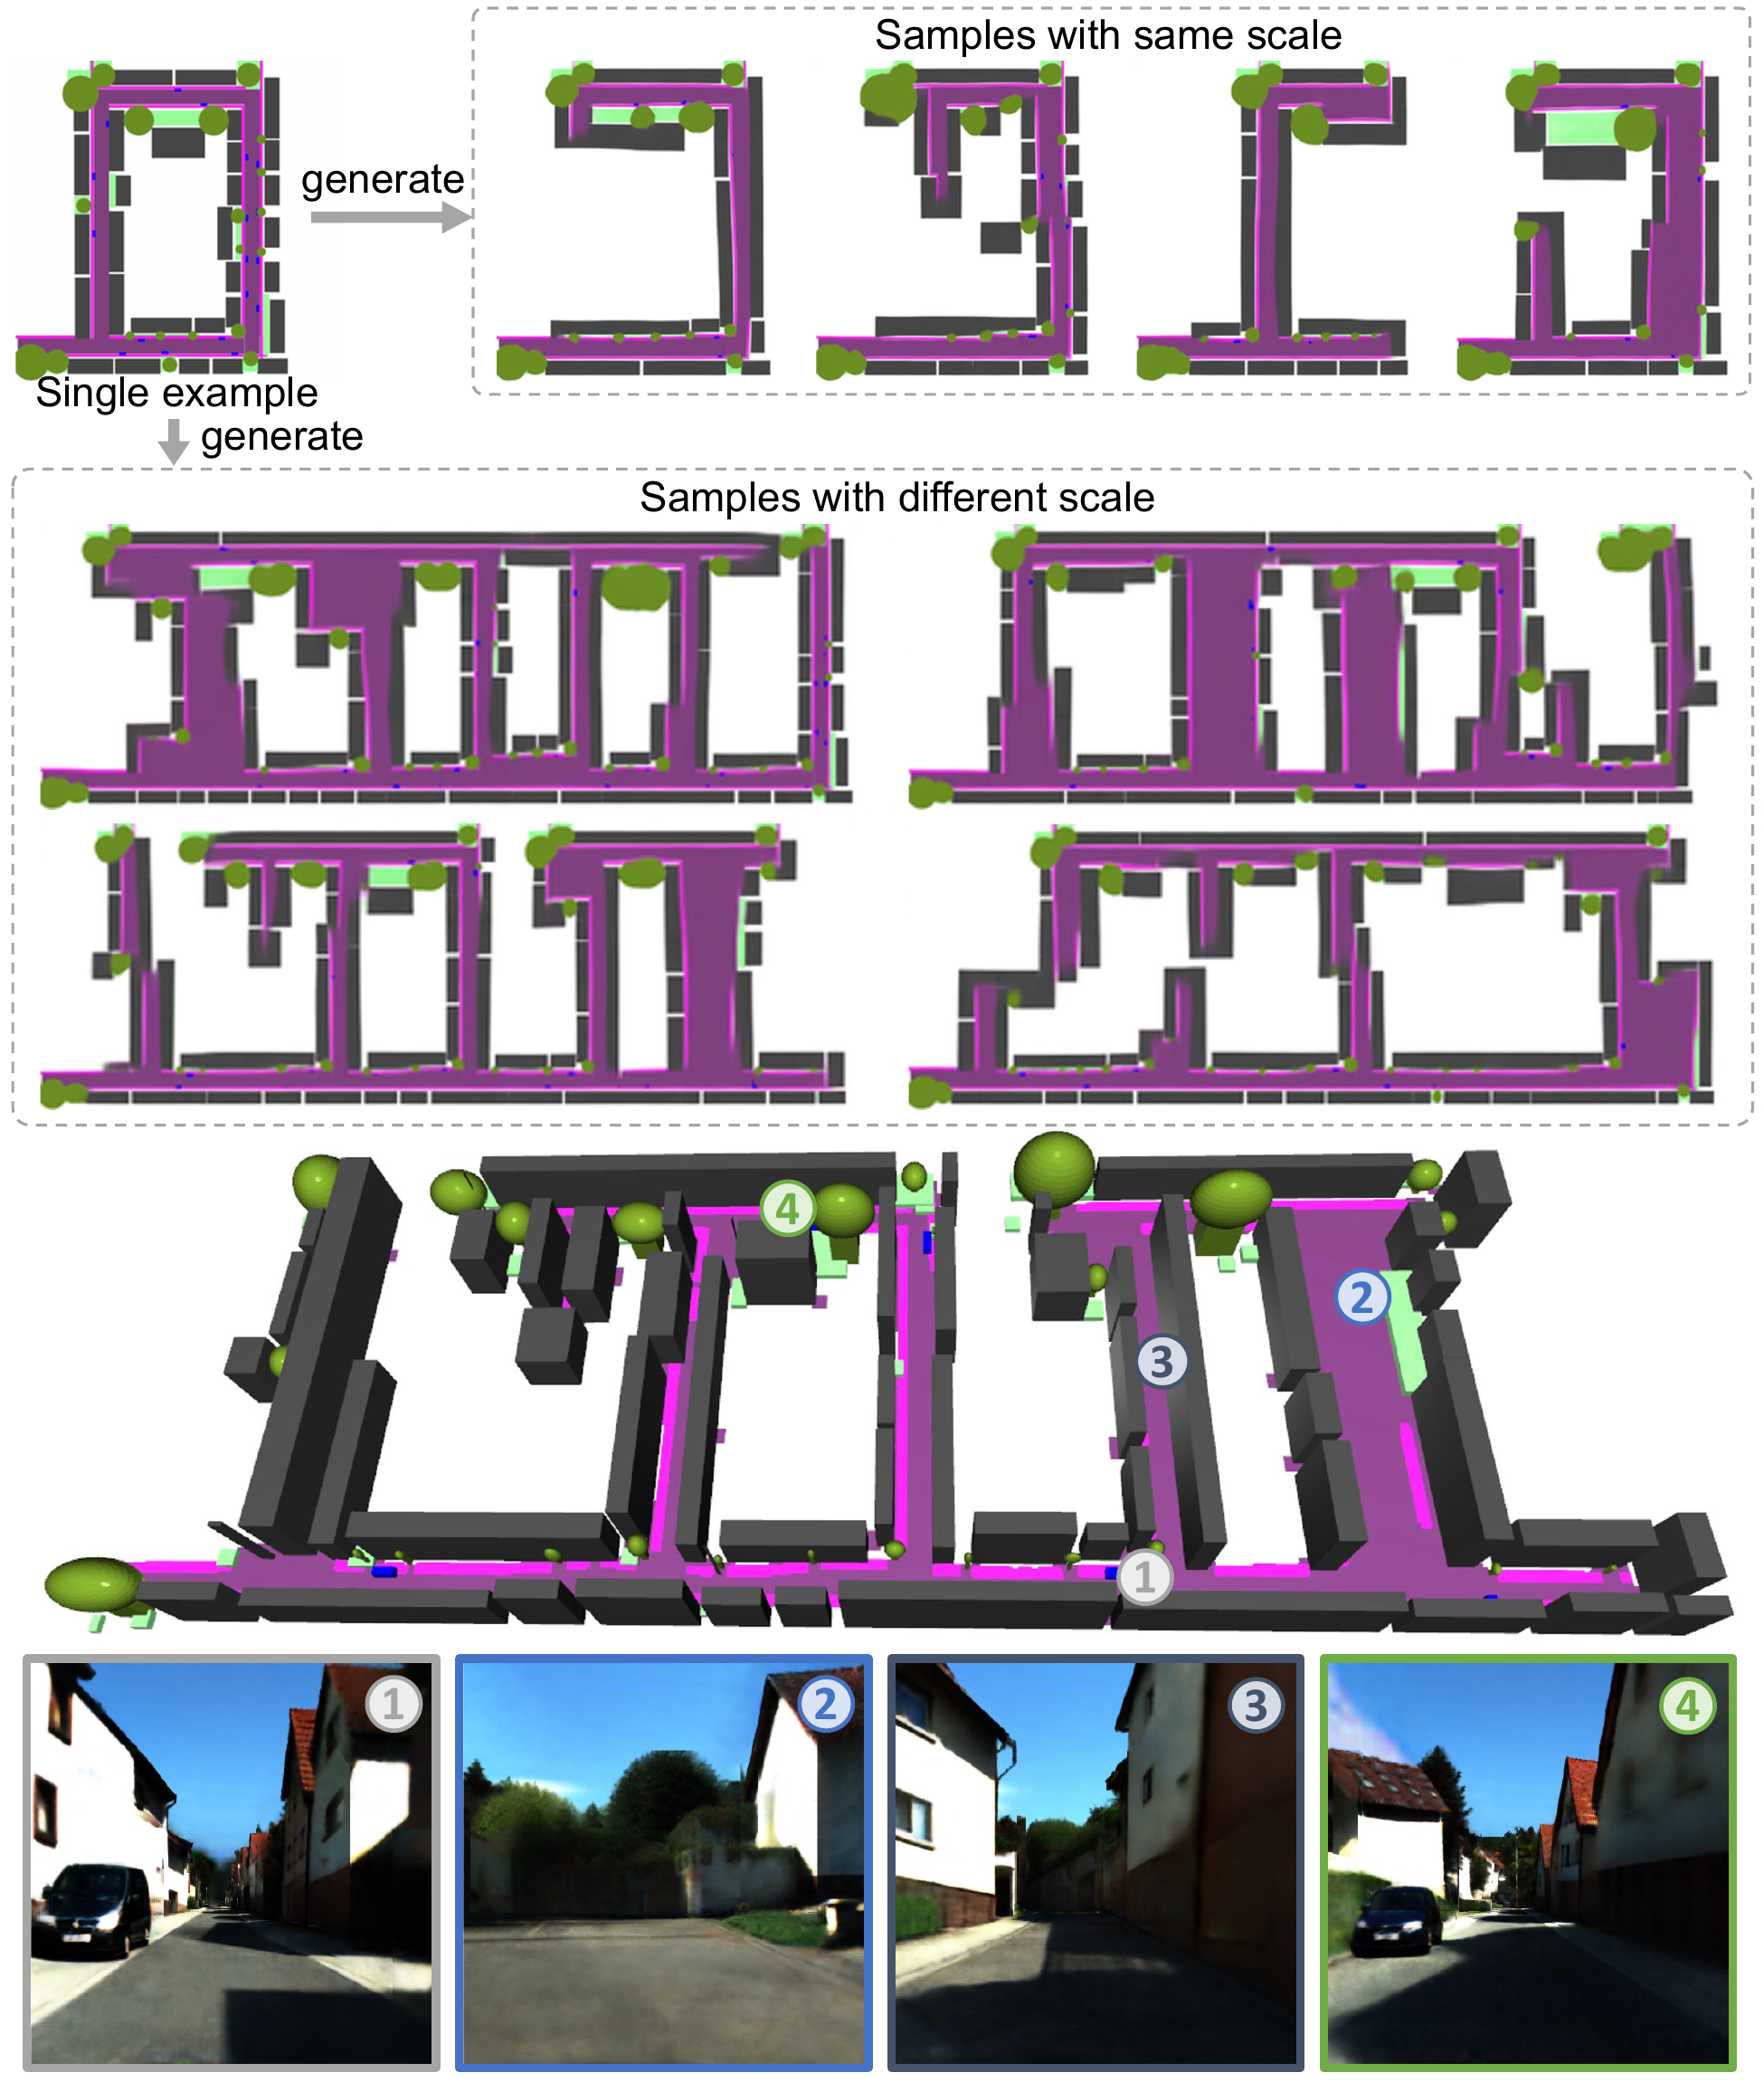}
% \vspace{-4ex}
\caption{\textbf{Automatic Layout Generation.} We present an alternative method for automatic 3D layout generation given a single example of the layout. In the top two rows, We display generated layouts with different scales and provide the corresponding 3D layout given the generated 2D sample in the third row. The rendering results of the generated scene are displayed in the bottom row.}\label{fig:sinddm}
% \vspace{-3ex}
\end{figure}
%and achieve automatic generation.
%Specifically, given that 3D layout of urban scenes can be a.
%By employing SinDDM, we can generate 
\section{Additional Experimental Results}
In this section, we provide additional ablation studies and more experimental results. Please refer to our supplementary video for more results.

\subsection{Additional Ablation Studies}
We provide more ablation studies to investigate the impact of individual components in our pipeline.

\begin{table}[ht]
\centering

\setlength\tabcolsep{10pt}
\footnotesize
\caption{Ablation studies on LG-VSD and layout-constrained sampling strategy on the KITTI-360 dataset.}
% KID is multiplied by $1000\times$ according to CC3D.
% \vspace{-3ex}
\begin{tabular}{l c c}
\toprule
\textbf{Method} & FID$\downarrow$ & KID$\downarrow$ \\
\midrule
w/o LG-VSD & 167.1 & 0.203 \\ % 121.0
w/o layout-constrained sampling & 143.5 & 0.148 \\ % 82.3
\midrule
Ours & \textbf{59.8} & \textbf{0.059} \\ % 58.6
\bottomrule
\end{tabular}
\label{tab:ablation}
% \vspace{-3ex}
\end{table}
\noindent\textbf{LG-VSD.} To further demonstrate the effectiveness of the proposed LG-VSD, we provide quantitative evaluations by using the diffusion model fine-tuned on KITTI-360 dataset to guide the generation process. According to Table~\ref{tab:ablation}, our LG-VSD significantly improves the performance, exhibiting much lower FID and KID on the KITTI-360 dataset.

\noindent\textbf{Layout-Constrained Sampling.} As mentioned before, the proposed pipeline would yield blurry results without the layout-constrained sampling strategy. As shown in Table~\ref{tab:ablation}, the FID and KID on the KITTI-360 dataset are significantly larger compared to those of our full model.

\noindent\textbf{CLIP Loss.} We perform experiments to verify the effectiveness of the CLIP loss. As shown in Fig.~\ref{fig:ablation_clip}, CLIP loss improves the details of generated scenes, enhancing the realism of the rendering results.

\begin{figure}[htbp] % 
\centering
\includegraphics[width=1\linewidth]{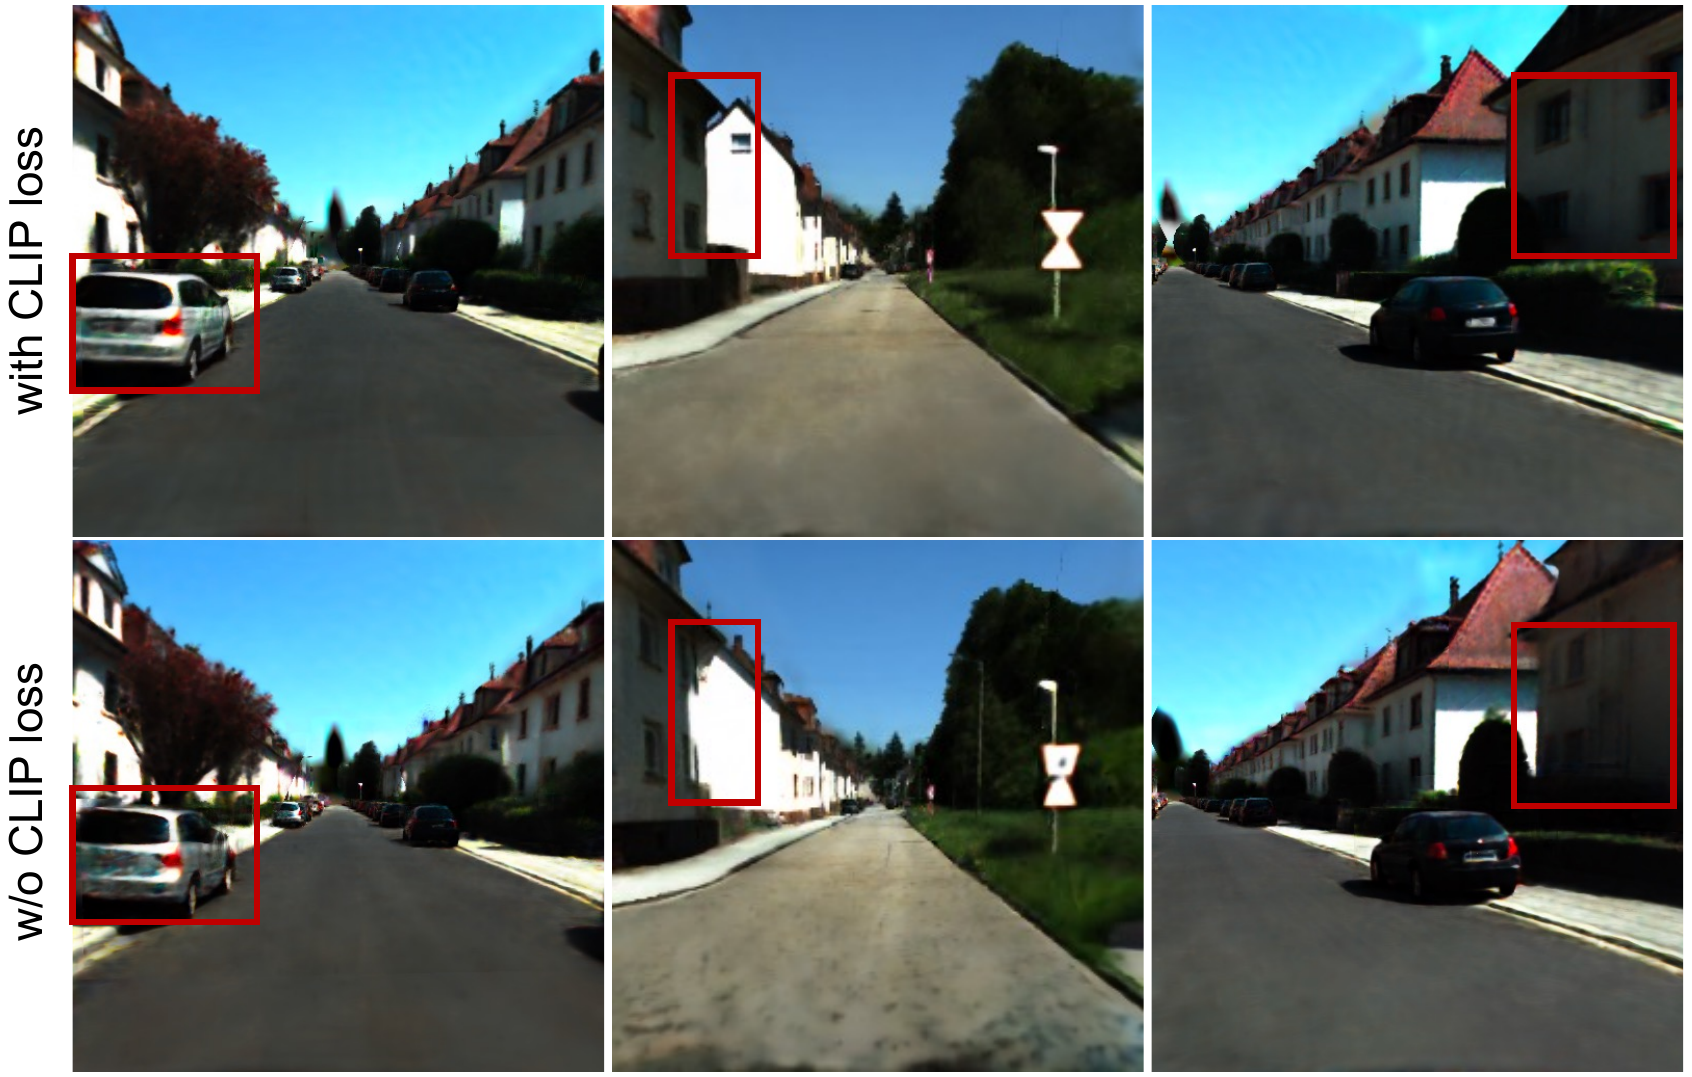}
% \vspace{-4ex}
\caption{\textbf{Ablation study on CLIP loss.} The introduction of CLIP loss enhances details of  generated scenes.}\label{fig:ablation_clip}
% \vspace{-3ex}
\end{figure}

\noindent\textbf{Layout-Aware Refinement.} We conduct experiments to investigate the influence of the layout-aware resampling process by refining the image using diffusion models without our layout conditions. According to the results in Fig.~\ref{fig:ablation_layout_aware}, the resampling process without layout conditions would mix up different instances, leading to structural distortions and blurry results.

\begin{figure}[htbp] % 
\centering
\includegraphics[width=1\linewidth]{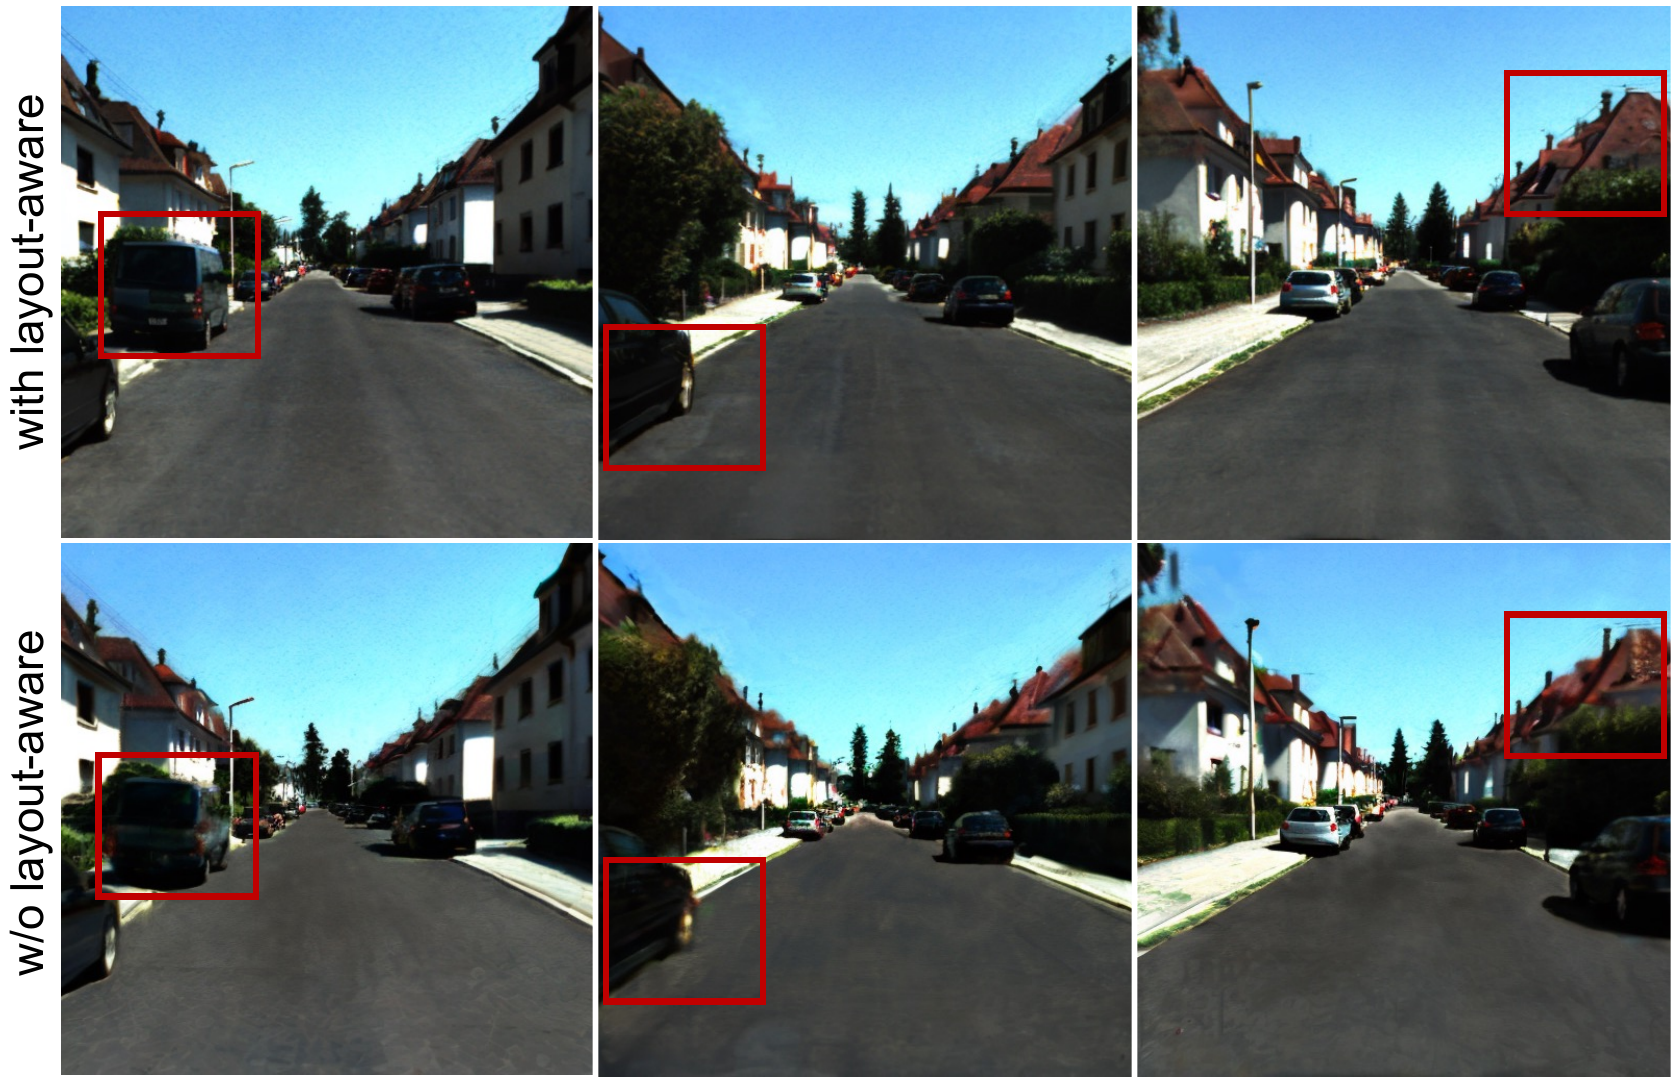}
% \vspace{-4ex}
\caption{\textbf{Ablation study on layout-aware refinement.} The layout-aware refinement process leads to better consistency. }\label{fig:ablation_layout_aware}
% \vspace{-3ex}
\end{figure}

\begin{figure*}[htbp] % 
\centering
\includegraphics[width=1\linewidth]{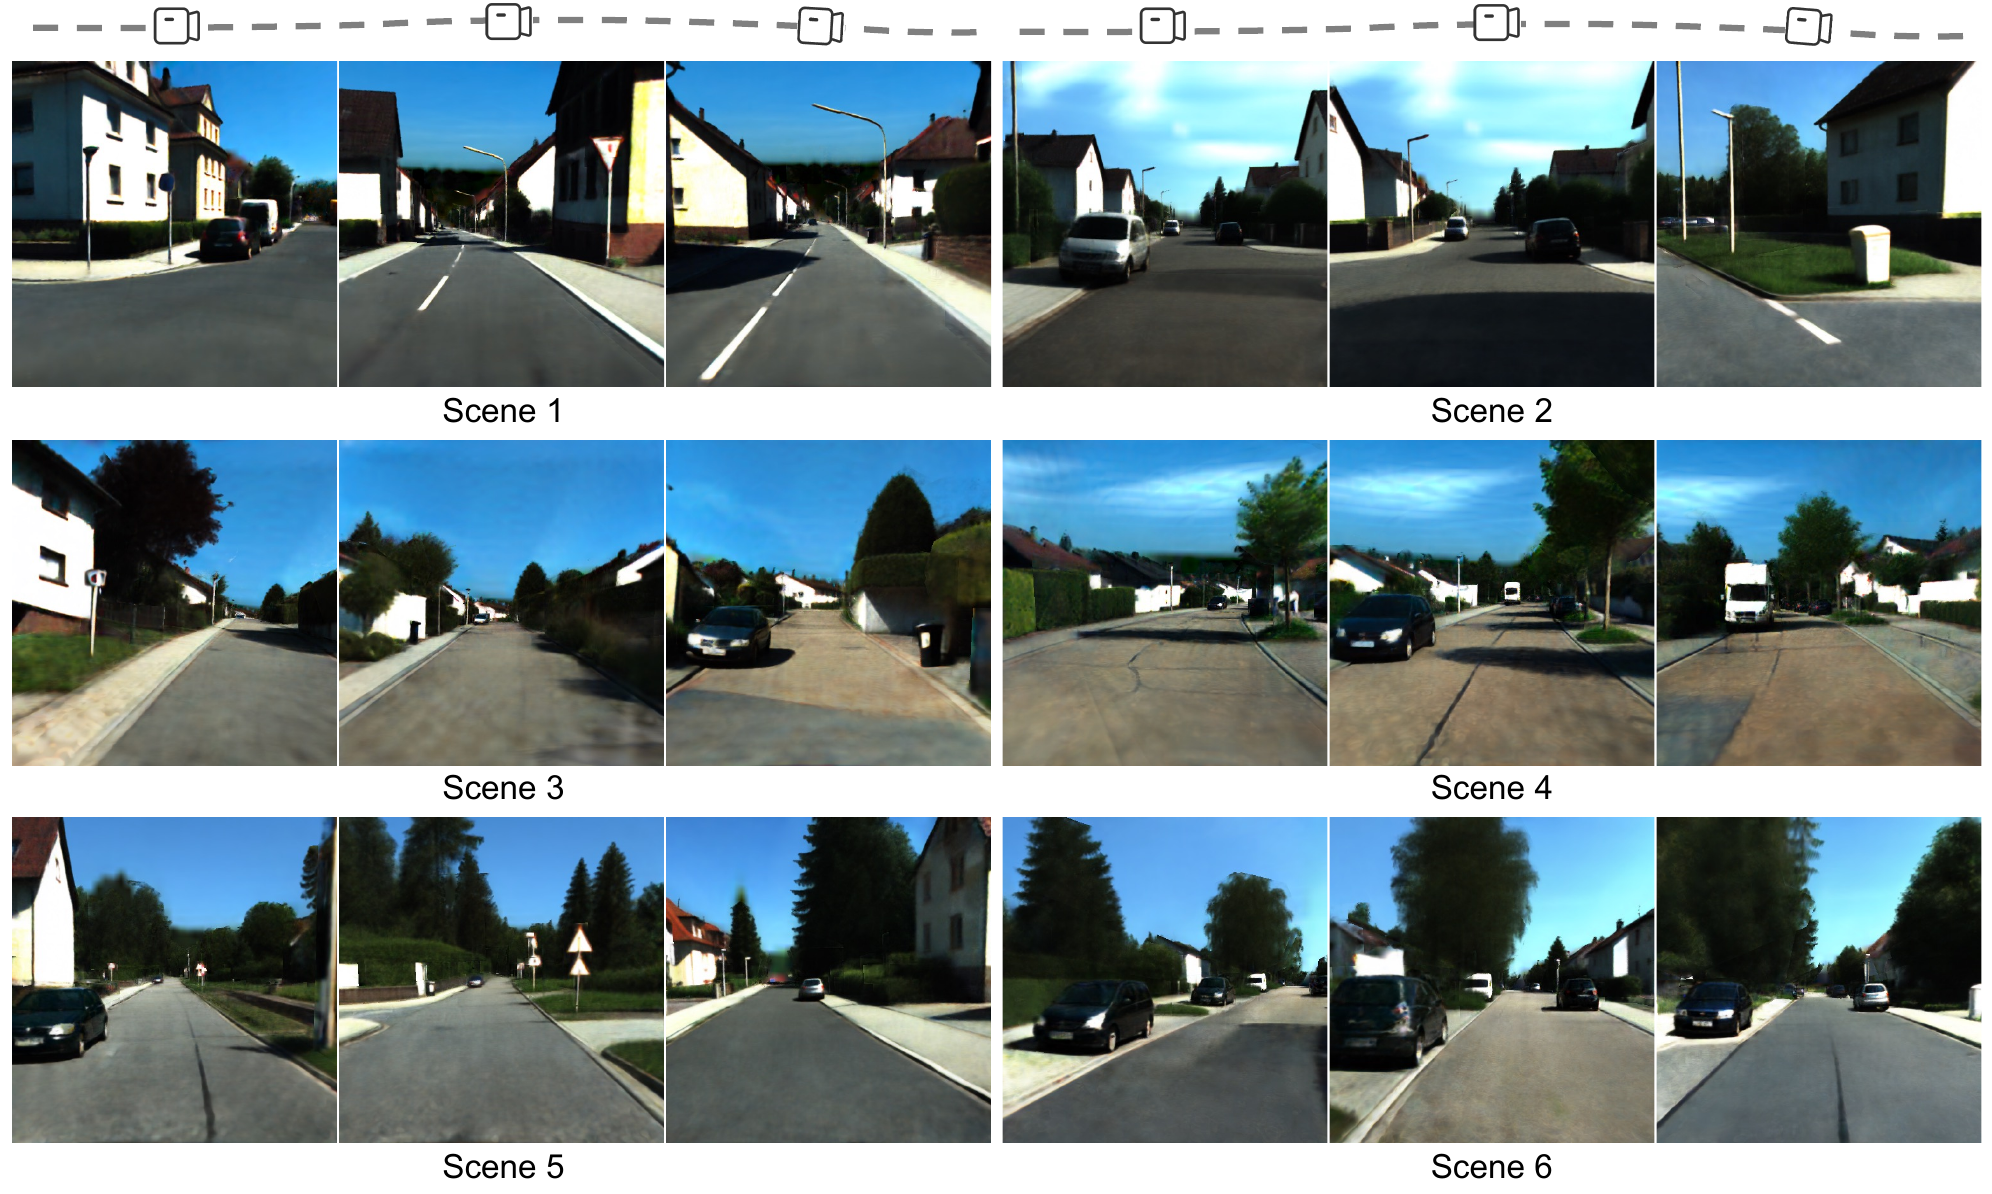}
\vspace{-4ex}
\caption{\textbf{More visualization results in KITTI-360 style.}}
\label{fig:morevis}
% \vspace{-3ex}
\end{figure*}

\begin{figure*}[htbp] % 
\centering
\includegraphics[width=1\linewidth]{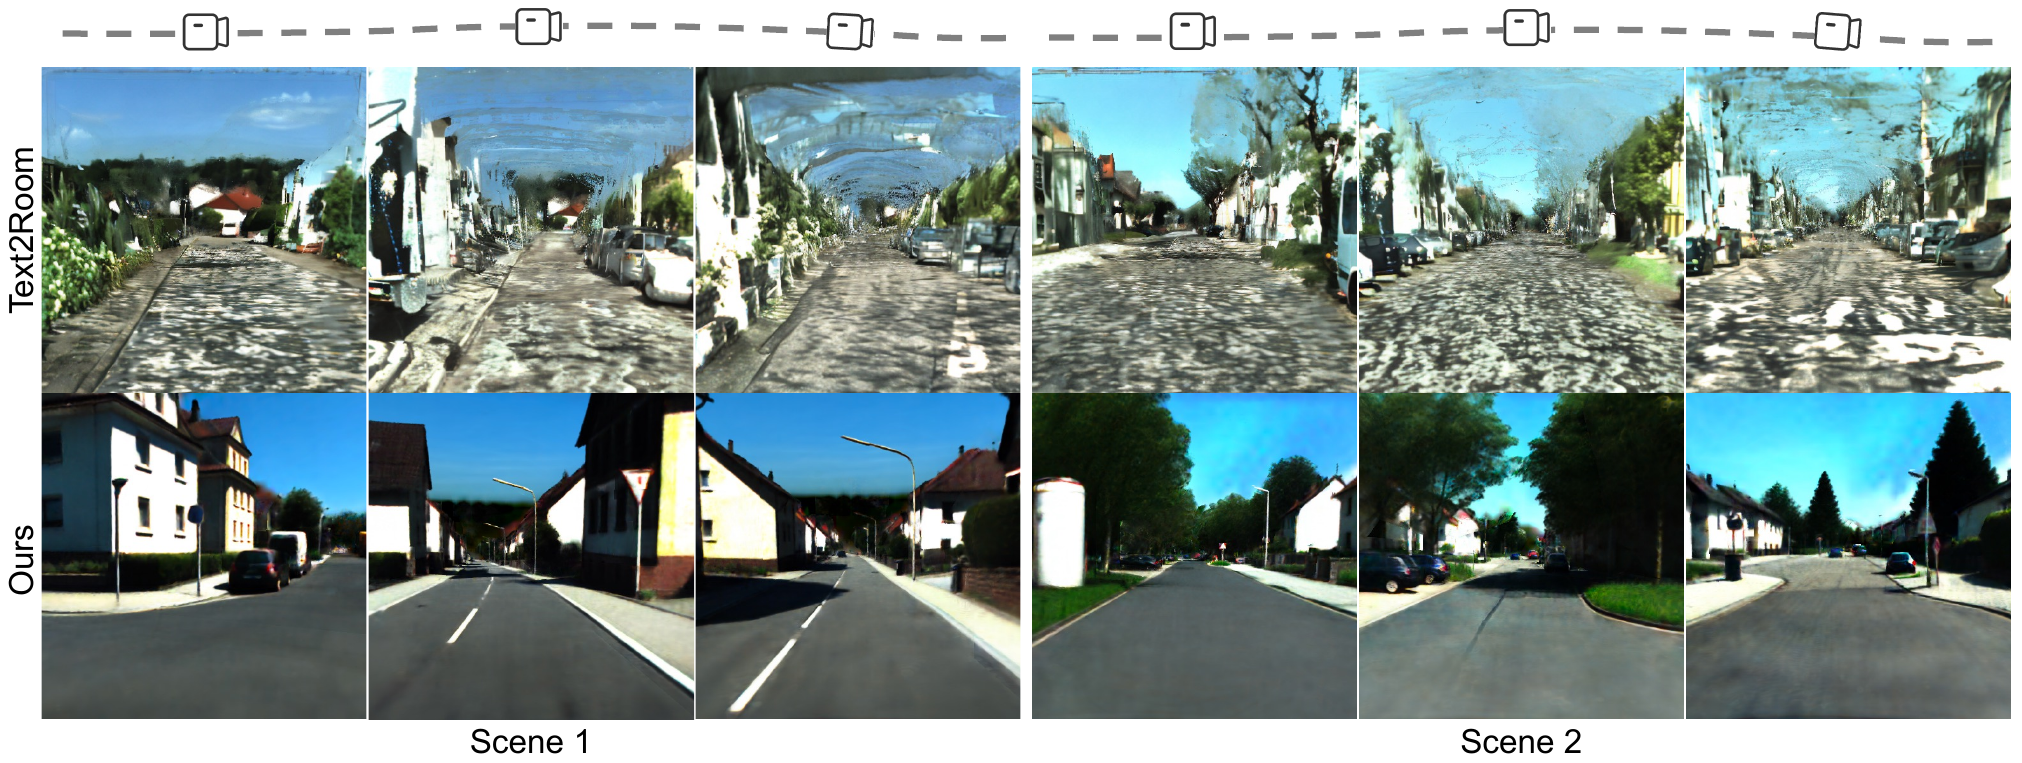}
% \vspace{-4ex}
\caption{\textbf{Qualitative comparison with Text2Room.} Text2Room would quickly degrade due to the cumulative errors during the incremental generation process.}\label{fig:text2room}
% \vspace{-3ex}
\end{figure*}

\begin{figure*}[htbp] % 
\centering
\includegraphics[width=0.95\textwidth]{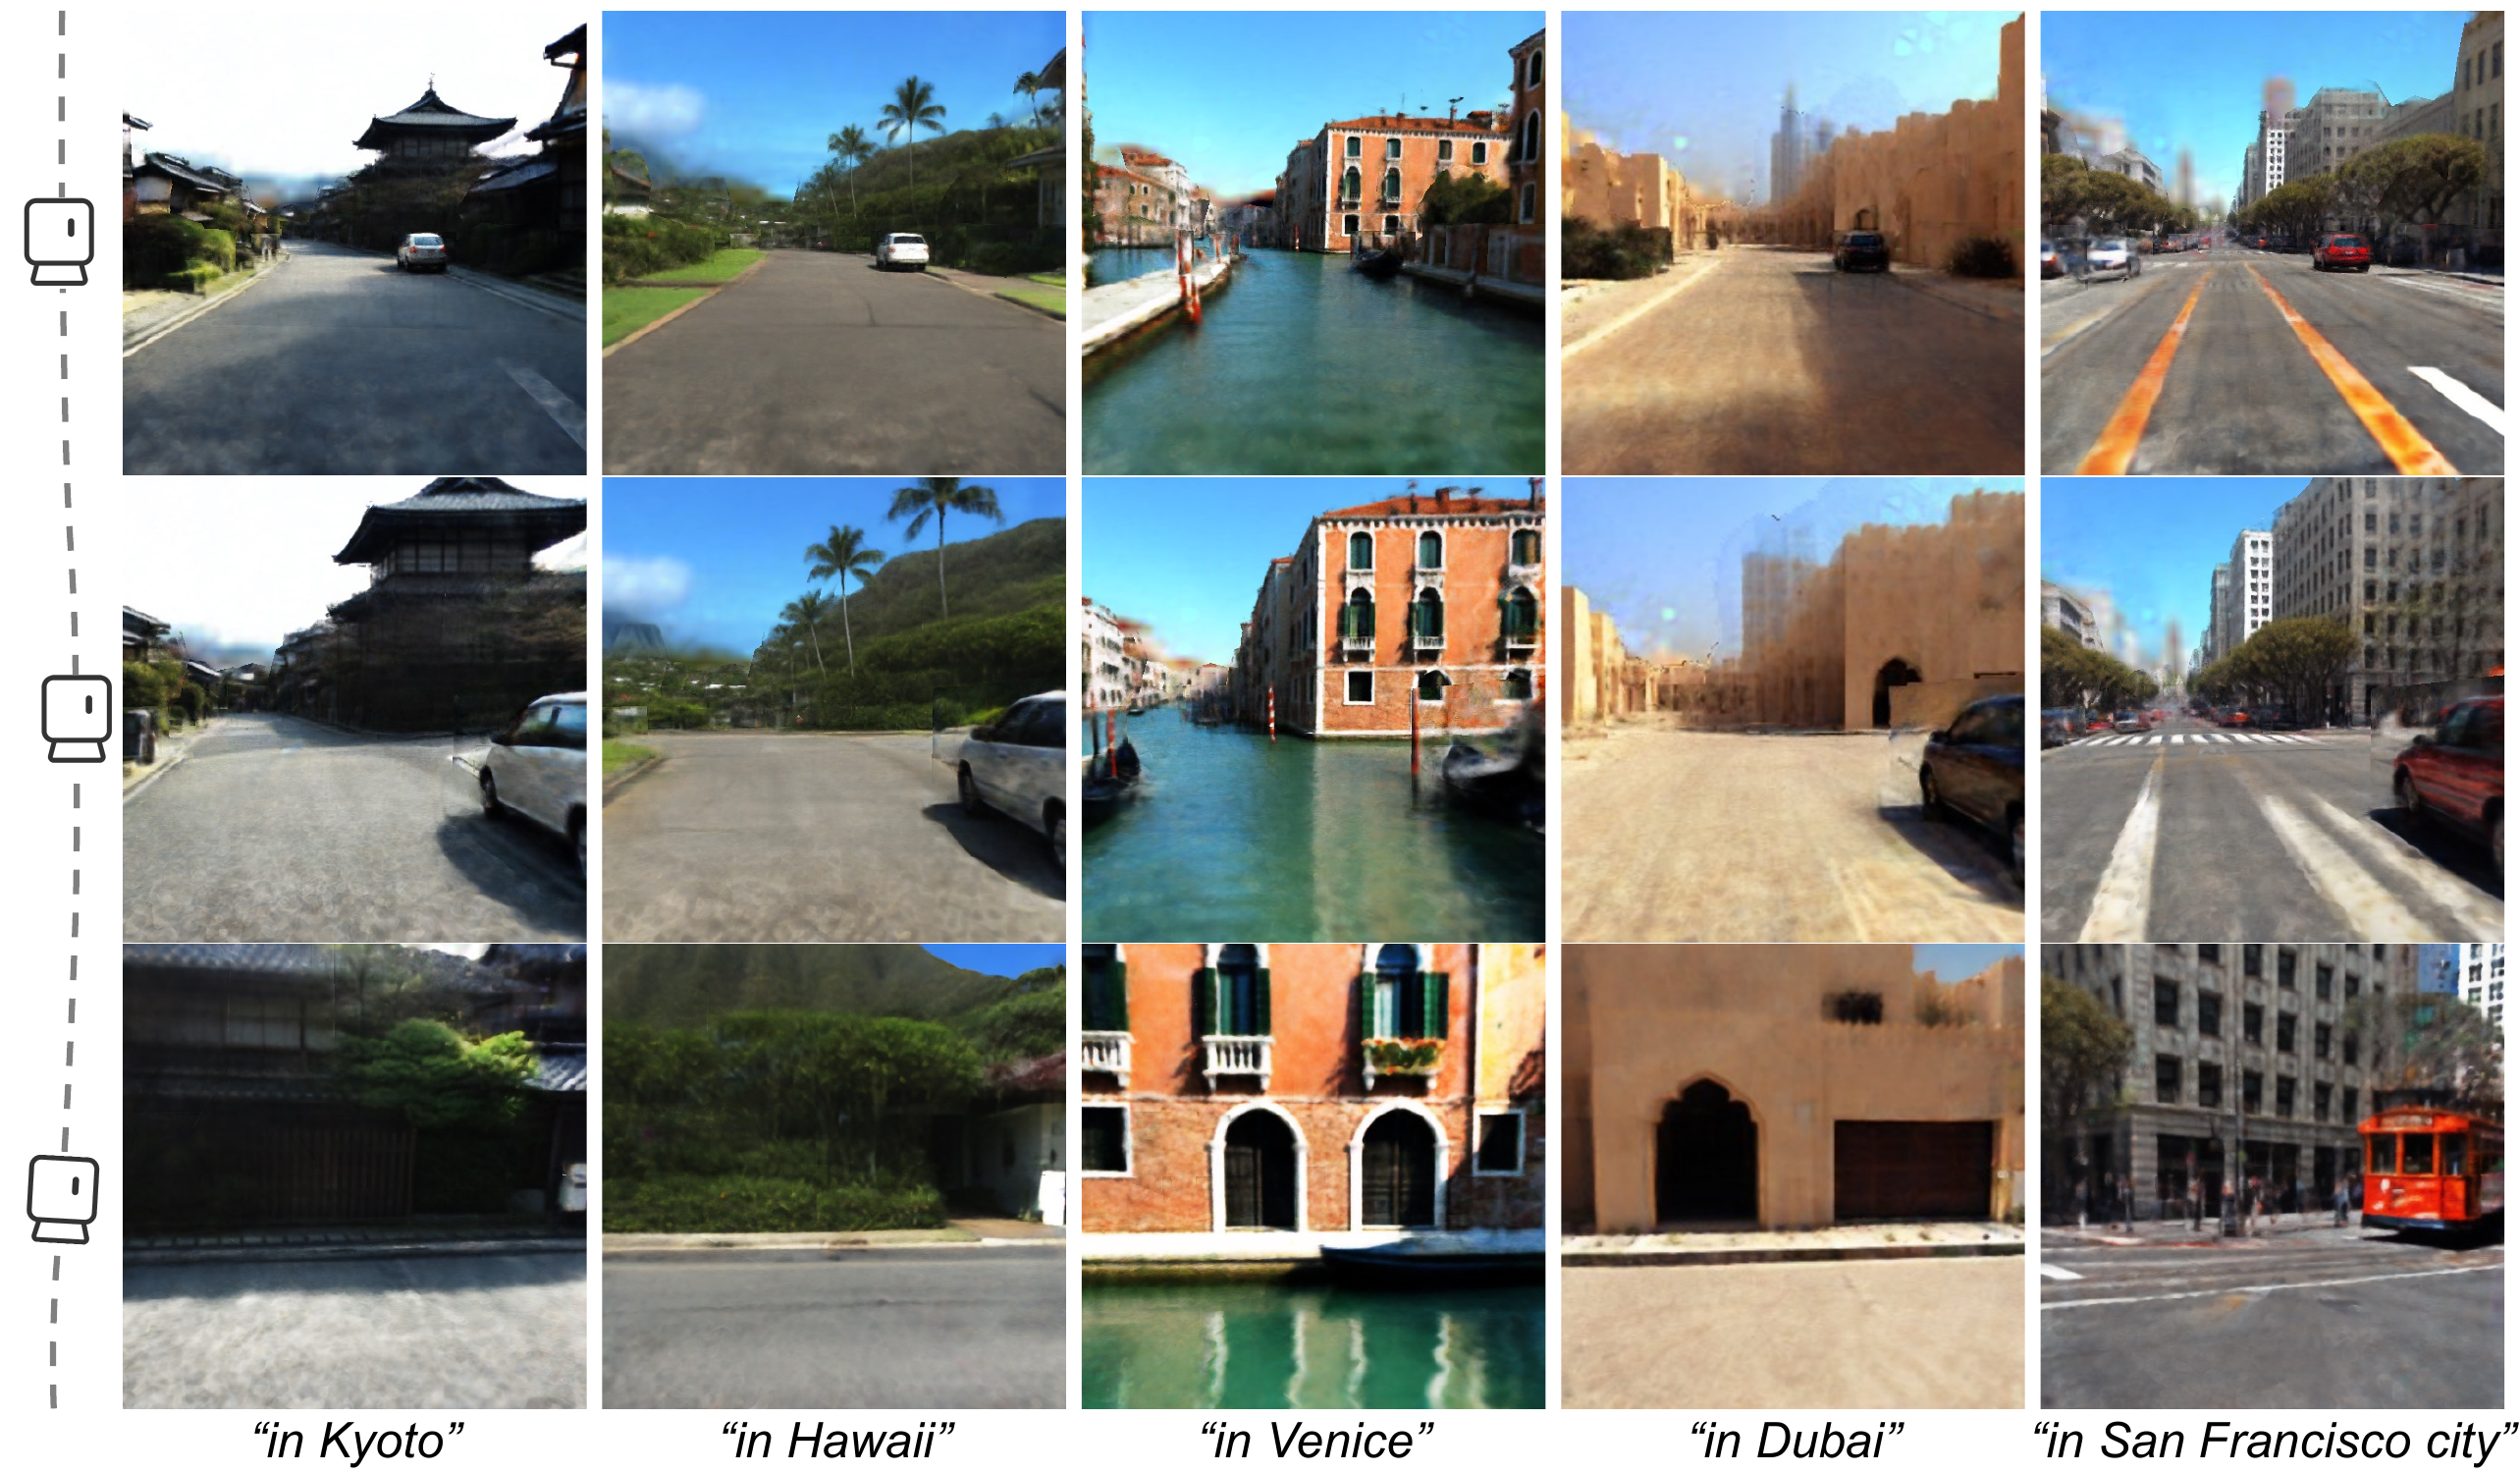}
% \vspace{-4ex}
\caption{\textbf{Transfer to other cities.} The generated urban scene can be transferred to different city styles given the text prompt by fine-tuning the generated hash grid.}
\label{fig:cityediting}
\vspace{-2ex}
\end{figure*}

\subsection{More Results}
We provide more experimental results to further explore the capabilities of our pipeline.

\noindent \textbf{More Visualization Results.} We provide more visualization results of our generated scenes in KITTI-360 style (shown in Fig.~\ref{fig:morevis}).

%{\color{red}(note: add 1-2sentences in each sub to analyse )}
\noindent \textbf{Comparison with Text2Room.} We further compare the proposed pipeline with Text2Room~\cite{Hollein_2023_ICCV}, which is initially designed for room-scale textured mesh generation. We integrate our pre-trained ControlNet into the inpainting model of Text2Room, enabling the generation of urban scenes based on our 3D layout information. According to the results in Fig.~\ref{fig:text2room}, this pipeline tends to  degrade rapidly under the influence of cumulative errors, resulting in a failure to produce valid results.

\noindent \textbf{Diversity with a Same Layout.} \textit{(1) Different city style}: As shown in Fig.~\ref{fig:cityediting}, we can further transfer the generated urban scene to various city styles by adding text prompt-based conditions (\eg, \textit{``in Kyoto"}, \textit{``in Hawaii"}, \etc), showcasing the complementary power of our layout-based guidance and text-to-image diffusion models. \textit{(2) Different random seeds}: We conduct experiments by employing different random seeds while maintaining the same layout to explore the diversity of our method. As shown in Fig.~\ref{fig:diversity}, given the same scene layout, the proposed pipeline can generate diverse scenes with elements (\eg, cars, buildings) that have different appearances and illumination. This demonstrates the diverse generation ability of the proposed model  -- where both the powers of layout and texture are brought into full play.

\begin{figure}[htbp] % 
\centering
\includegraphics[width=1\linewidth]{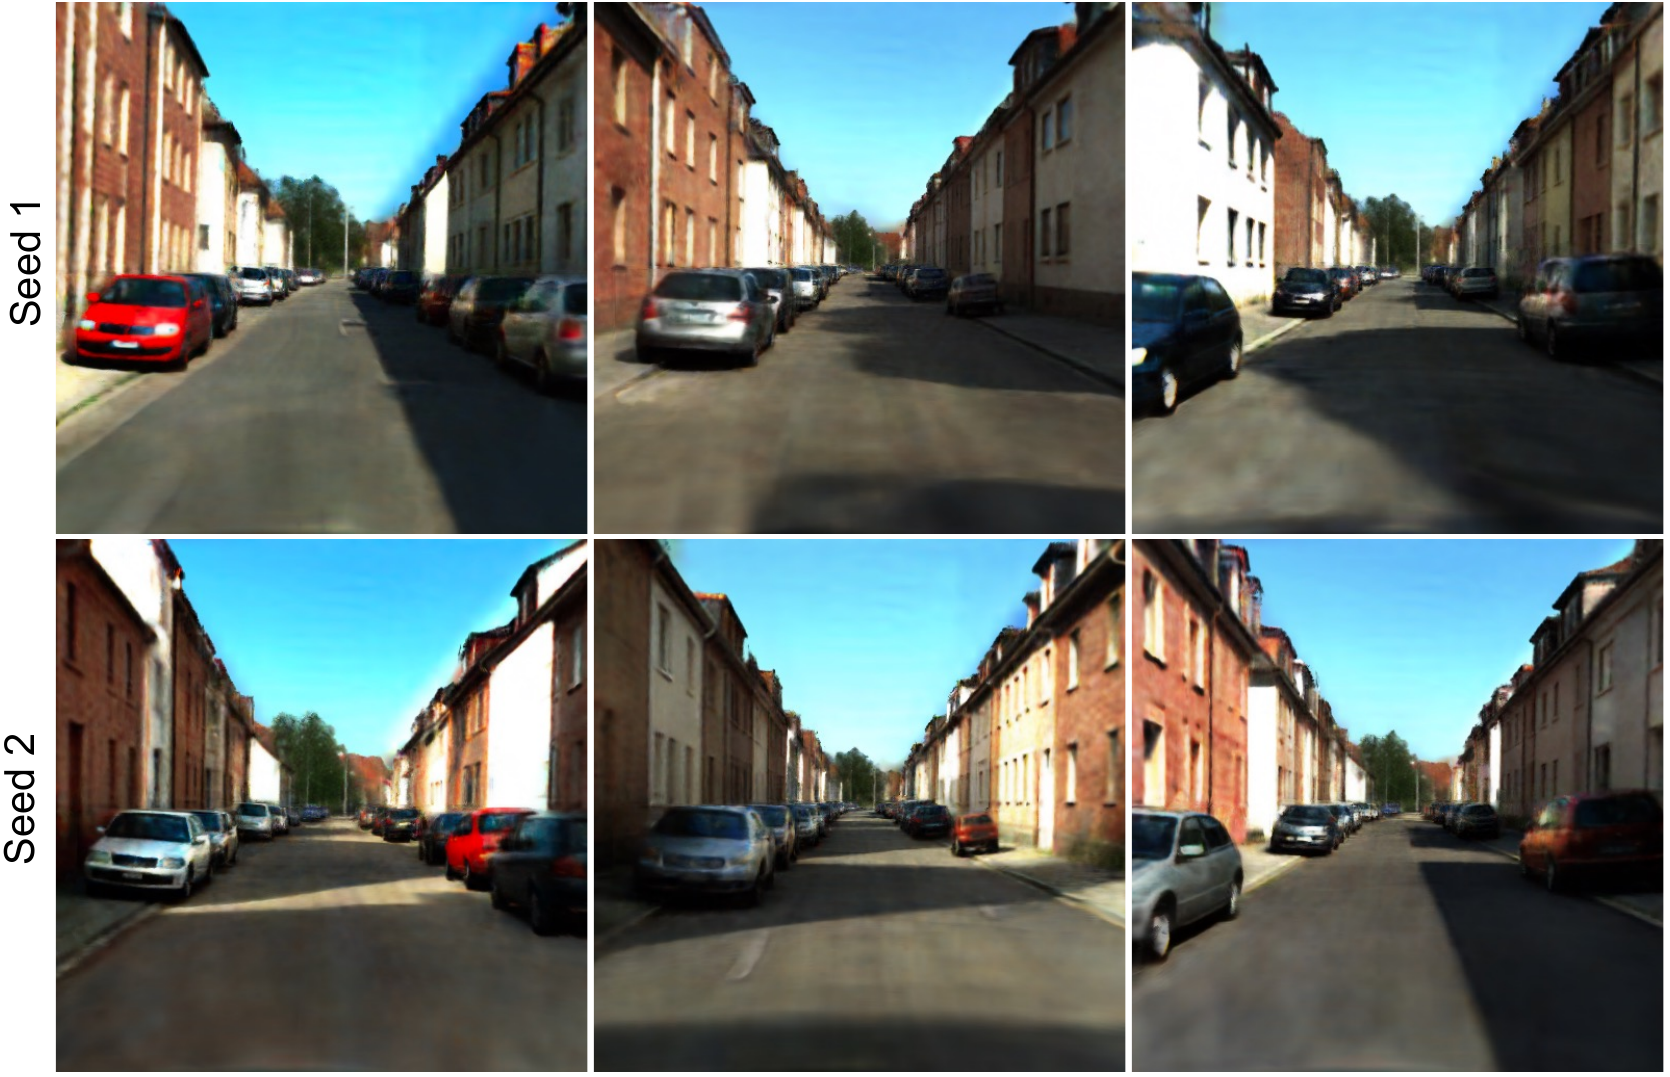}
% \vspace{-4ex}
\caption{\textbf{Generated results with different random seeds.} We display the generated scenes with two different random seeds given the same scene layout.}\label{fig:diversity}
% \vspace{-3ex}
\end{figure}

% {\color{red}(note: same layout in three-level -- (1)seed (2)car color/material (3) diff text style- style/building style )}

%\section{Additional Experimental Results}{\color{red}{note: 1.which exp is quantitative?2.subdiv the section into two sec}

\noindent \textbf{Large Camera View Shifting.} As shown in Fig.~\ref{fig:viewshifting}, we display the rendering results by rotating the camera from $-45\deg$ to $45\deg$. Owing to the high 3D consistency, the generated scene demonstrates strong robustness against large camera view shifting.

\begin{figure}[htbp] % 
\centering
\includegraphics[width=1\linewidth]{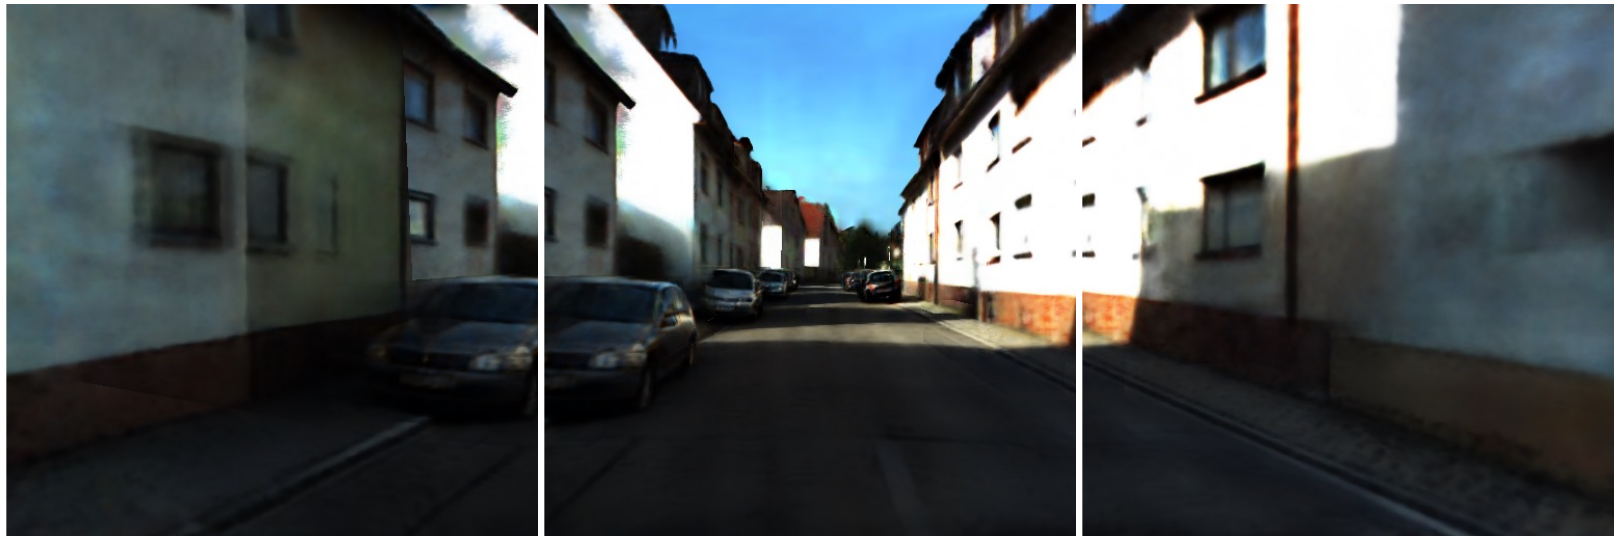}
% \vspace{-4ex}
\caption{\textbf{Large camera view shifting.} The camera rotates from $-45\deg$ to $45\deg$ from left to right.}\label{fig:viewshifting}
% \vspace{-3ex}
\end{figure}

\begin{figure}[htbp] % 
\centering
\includegraphics[width=1\linewidth]{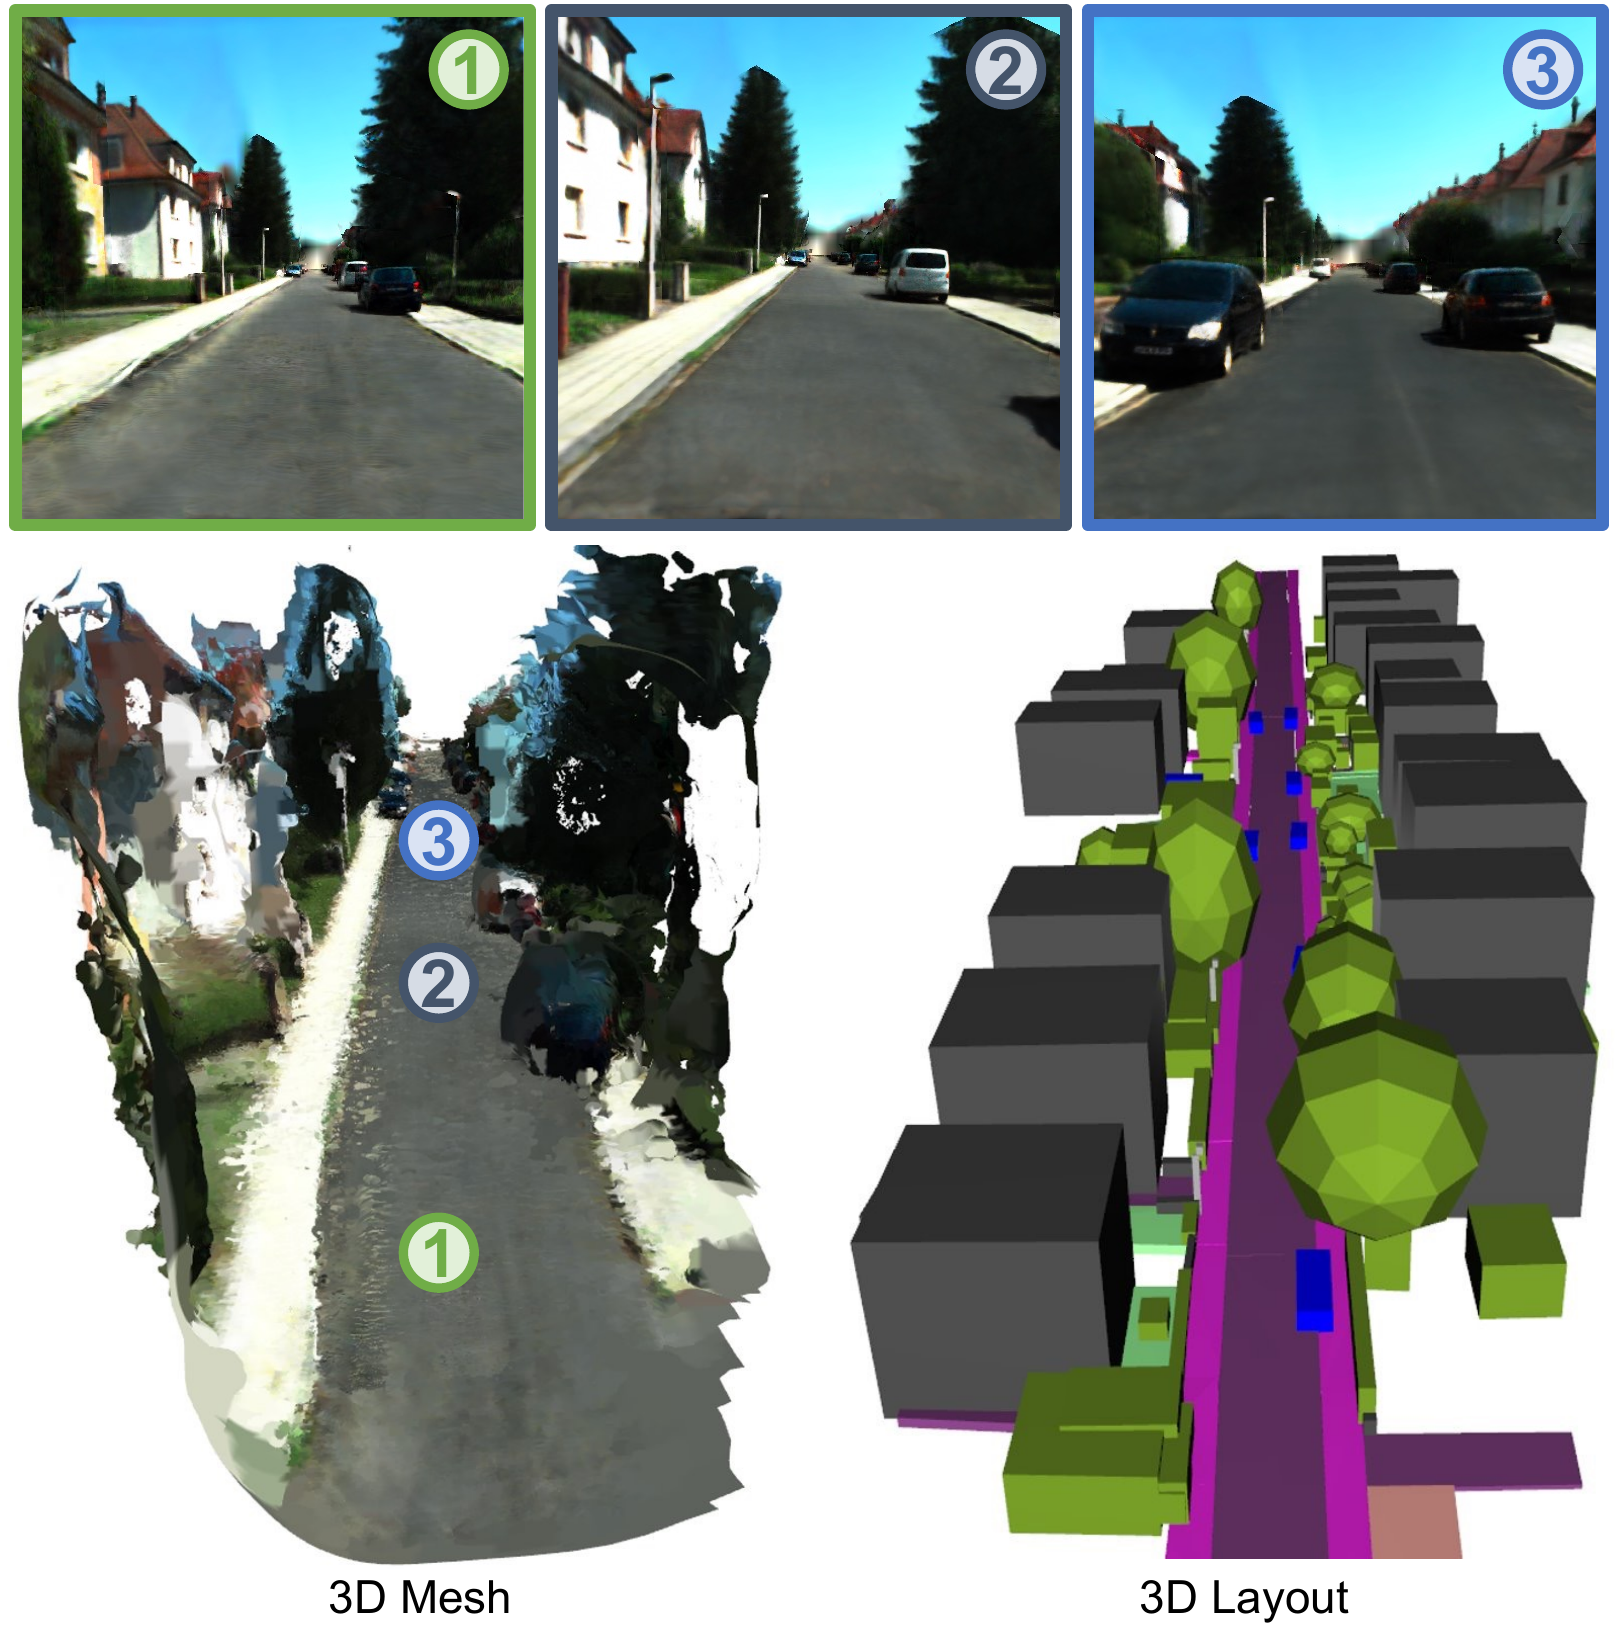}
% \vspace{-4ex}

\caption{\textbf{3D mesh visualization.} We extract a 3D triangle mesh from the generated scene and provide rendered 2D images from corresponding camera poses.}
\label{fig:3dresults}
% \vspace{-3ex}
\end{figure}

% \noindent \textbf{Transfer to Other Cities.}  As shown in Fig.~\ref{fig:cityediting}, we can further transfer the generated urban scene to different city styles via adding a text prompt (\eg, \textit{``in Kyoto"}, \textit{``in Hawaii"}, \etc), showing the complementary power of our layout-based guidance and text-to-image diffusion models.

% \noindent \textbf{Ablation on CLIP Loss.}

% \noindent \textbf{Ablation on Depth Condition.}

% \noindent \textbf{Ablation on Layout-Aware Refinement.}

\noindent \textbf{3D Results.} To further explore the 3D consistency of the generated scene, we extract a triangle mesh from the generated hash grid and display the results in Fig.~\ref{fig:3dresults}. The 3D triangle mesh reveals the consistent 3D structures of the generated scene.

% {\color{red}(note: why not 6 scenes, and each has 6frames?)}

% \subsection{large camera view shifting}
% \subsection{style editing in long seq}
% \subsection{Transfer to other city style?}
% \subsection{Point Cloud Results}

% \subsection{Layout-Aware Refinement}

% \subsection{Gaussian Splatting?}

% \subsection{CLIP loss}

% \subsection{Depth Condition}

% \subsection{Detailed Prior}

\section{Potential Negative Societal Impact} This paper presents a novel framework for large-scale 3D urban scene generation. We believe this technology has a positive impact on society. For example, our pipeline can be employed to build simulation environments for autonomous driving. However, due to the high quality and controllability of the proposed pipeline, there is potential for application in areas with negative social impacts, such as fake news generation. To address this concern, we may add watermarks to generated results to discourage negative applications.

%there is no guarantee that it could not be used in applications with negative social impacts. For example, this technique can be applied to synthesize fake scenes, which can further be used to generate fake events and news. 

% Ablation studies: detailed prior, CLIP loss, guided refinement, depth condition

% Point cloud rep

% single example-based layout generation

% Gaussian splatting:

% \section{Rationale}
% \label{sec:rationale}
% % 
% Having the supplementary compiled together with the main paper means that:
% % 
% \begin{itemize}
% \item The supplementary can back-reference sections of the main paper, for example, we can refer to \cref{sec:intro};
% \item The main paper can forward reference sub-sections within the supplementary explicitly (e.g. referring to a particular experiment); 
% \item When submitted to arXiv, the supplementary will already included at the end of the paper.
% \end{itemize}
% % 
% To split the supplementary pages from the main paper, you can use \href{https://support.apple.com/en-ca/guide/preview/prvw11793/mac#:~:text=Delete%20a%20page%20from%20a,or%20choose%20Edit%20%3E%20Delete).}{Preview (on macOS)}, \href{https://www.adobe.com/acrobat/how-to/delete-pages-from-pdf.html#:~:text=Choose%20%E2%80%9CTools%E2%80%9D%20%3E%20%E2%80%9COrganize,or%20pages%20from%20the%20file.}{Adobe Acrobat} (on all OSs), as well as \href{https://superuser.com/questions/517986/is-it-possible-to-delete-some-pages-of-a-pdf-document}{command line tools}.
